# Supplementary material for: Stable and efficient Petrov-Galerkin methods for a kinetic Fokker-Planck equation
Source: arXiv:2010.15784 ancillary file (2021-04-12)
Supplement: Supplementary file 1 [file fp_supplement.pdf]

# SUPPLEMENTARY MATERIALS: STABLE AND EFFICIENT PETROV-GALERKIN METHODS FOR A KINETIC FOKKER-PLANCK EQUATION

JULIA BRUNKEN AND KATHRIN SMETANA

## S1. Proof of proposition 3.1

*Proof of proposition 3.1.* The claim is only a slight variant of [S1, Prop. 7.1], where the result is shown for the space

$$\tilde{H}^1_{\mathrm{FP}}(\Omega) := \{p \in L^2(\Omega_{t,x}; \tilde{V}) \,:\, \partial_t p - v \cdot \nabla_x p \in L^2(\Omega_{t,x}; \tilde{V}')\} \tag{S1}$$

with $\tilde{V} = H^1_\gamma(\mathbb{R}^d)$ being the Sobolev space on $\mathbb{R}^d$ with standard Gaussian measure. The space $\tilde{H}^1_{\mathrm{FP}}(\Omega)$ is used to describe a Fokker-Planck equation similar to (2), but on $\tilde{\Omega}_v = \mathbb{R}^d$ and with a reverse sign for the transport term. We will therefore reuse the proofs of [S1, Prop. 7.1] (and [S1, Prop. 2.2], which treats the time-independent case) and modify only the parts dependent on $V$ and $\Omega_v$.

In step 1 of the proofs it is shown that we can assume without loss of generality that for every $z := (t, x) \in \Omega_{t,x} \subset \mathbb{R}^{d+1}$ and $\varepsilon \in (0, 1]$ we have $B((1-\varepsilon)z, \varepsilon) \subset \Omega_{t,x}$, where $B(z, r)$ is the open ball with radius $r$ around $z$.

Let then $f \in H^1_{\mathrm{FP}}(\Omega)$. As in step 2 of the proofs we take $\zeta \in C_0^\infty(\mathbb{R}^{d+1}, \mathbb{R})$ as a smooth function with compact support in $B(0, 1)$ such that $\int_{\mathbb{R}^{d+1}} \zeta = 1$. For each $\varepsilon > 0$ and $z \in \mathbb{R}^{d+1}$ we write $\zeta_\varepsilon(z) := \varepsilon^{-(d+1)}\zeta(\varepsilon^{-1}z)$, and define for $\varepsilon \in (0, \frac{1}{2}]$, $z \in \Omega_{t,x}$, and $v \in \Omega_v$ the mollification $f_\varepsilon(z, v) := \int_{\mathbb{R}^{d+1}} f((1-\varepsilon)z + z', v)\zeta_\varepsilon(z')\,\mathrm{d}z'$, so that we have $f_\varepsilon \in C^\infty(\bar{\Omega}_{t,x}; V)$. We may then show completely analogous to step 2 of the proofs of [S1, Prop. 2.2 and 7.1] that $f$ belongs to the closed convex hull of the set $\{f_\varepsilon : \varepsilon \in (0, \frac{1}{2}]\}$ by just changing the spaces of all dual pairings and norms from $\tilde{V} = H^1_\gamma(\mathbb{R}^d)$ to $V = H^1(S^{d-1})$ and from $L^2_\gamma(\mathbb{R}^d)$ to $L^2(S^{d-1})$.

It then remains to be shown that for fixed $\varepsilon \in (0, \frac{1}{2}]$ the function $f_\varepsilon$ belongs to $\mathrm{clos}_{\|\cdot\|_{H^1_{\mathrm{FP}}}} C^\infty(\bar{\Omega}_{t,x} \times \Omega_v)$ by approximating $f_\varepsilon$ also in the $v$-variable.

We construct a basis of $V = H^1(\Omega_v)$ that is contained in $C^\infty(\Omega_v)$: Since $V$ as a subspace of $L^2(\Omega_v)$ is separable and $C^\infty(\Omega_v) \subset V$, there exists a dense countable set in $(C^\infty(\Omega_v), \|\cdot\|_V)$, from which we can obtain an orthonormal basis $(\psi_i)_{i\in\mathbb{N}}$ by the Gram-Schmidt algorithm. Since $\mathrm{span}(\psi_i)_{i\in\mathbb{N}}$ is dense in $C^\infty(\Omega_v)$ which is again dense in $V$ (cf. e.g. [S9, Thm 2.4, p. 25]), $(\psi_i)_{i\in\mathbb{N}}$ is also an orthonormal basis of $V$.

For $k \in \mathbb{N}$, we define $f_{\varepsilon,k} : \Omega_{t,x} \times \Omega_v \to \mathbb{R}$ as $f_{\varepsilon,k}(z, v) := \sum_{i=1}^k (f_\varepsilon(z, \cdot), \psi_i)_V \psi_i(v)$.

*Date*: April 12, 2021.

The work of Julia Brunken was supported by the German Federal Ministry of Education and Research under grant BMBF 05M2016 - GlioMaTh and by the Deutsche Forschungsgemeinschaft (DFG, German Research Foundation) under Germany's Excellence Strategy EXC 2044 –390685587, Mathematics Münster: Dynamics–Geometry–Structure.

Since we have $f_\varepsilon \in C^\infty(\bar{\Omega}_{t,x}; V)$, the map $z \mapsto (f_\varepsilon(z, \cdot), \psi_i)_V$ is in $C^\infty(\bar{\Omega}_{t,x})$. As $\psi_i \in C^\infty(\Omega_v)$ for all $i \in \mathbb{N}$, we have $f_{\varepsilon,k} \in C^\infty(\bar{\Omega}_{t,x} \times \Omega_v)$ for all $k \in \mathbb{N}$.

Next, we compute $\lim_{k\to\infty} \|f_\varepsilon - f_{\varepsilon,k}\|_{L^2(\Omega_{t,x};V)}$. First, fix $z \in \bar{\Omega}_{t,x}$. Since $(\psi_i)_{i\in\mathbb{N}}$ is an orthonormal basis of $V$ we have $f_\varepsilon(z) = \sum_{i=1}^{\infty} (f_\varepsilon(z), \psi_i)_V \psi_i$ and thus

$$\|f_\varepsilon(z) - f_{\varepsilon,k}(z)\|_V = \left\| \sum_{i=k+1}^{\infty} (f_\varepsilon(z), \psi_i)_V \psi_i \right\|_V = \sum_{i=k+1}^{\infty} (f_\varepsilon(z), \psi_i)_V^2 \overset{k\to\infty}{\to} 0.$$

As this holds for all $z \in \bar{\Omega}_{t,x}$ and $\|f_\varepsilon(z) - f_{\varepsilon,k}(z)\|_V \le 2\|f_\varepsilon(z)\|_V$, we obtain by the dominated convergence theorem that $\lim_{k\to\infty} \|f_\varepsilon - f_{\varepsilon,k}\|_{L^2(\Omega_{t,x};V)} = 0$. To determine $\lim_{k\to\infty} \|\binom{1}{v} \cdot \nabla_z (f_\varepsilon - f_{\varepsilon,k})\|_{L^2(\Omega_{t,x};V')}$, we first consider the partial derivatives separately: Since $f_\varepsilon \in C^\infty(\bar{\Omega}_{t,x}; V)$, all first $z$-partial derivatives of $f_\varepsilon$ lie in $L^2(\Omega_{t,x}; V)$ and we know that

$$\|\partial_{z_j} f_\varepsilon(z) - \partial_{z_j} f_{\varepsilon,k}(z)\|_V = \| \sum_{i=k+1}^{\infty} (\partial_{z_j} f_\varepsilon(z), \psi_i)_V \psi_i \|_V \overset{k\to\infty}{\to} 0$$

for $j = 1, \ldots, d+1$, and all $z \in \bar{\Omega}_{t,x}$. Since $|\binom{1}{v}|$ is bounded on $\Omega_v = S^{d-1}$, we thus have

$$\begin{aligned}\|\tbinom{1}{v} \cdot \nabla_z (f_\varepsilon(z) - f_{\varepsilon,k}(z))\|_{L^2(\Omega_v)} &\le \sum_{j=1}^{d+1} \|\tbinom{1}{v}_j\|_{L^\infty(\Omega_v)} \|\partial_{z_j} f_\varepsilon(z) - \partial_{z_j} f_{\varepsilon,k}(z)\|_{L^2(\Omega_v)} \\ &\le \sum_{j=1}^{d+1} \|\tbinom{1}{v}_j\|_{L^\infty(\Omega_v)} \|\partial_{z_j} f_\varepsilon(z) - \partial_{z_j} f_{\varepsilon,k}(z)\|_V \overset{k\to\infty}{\to} 0,\end{aligned}$$

and again by the dominated convergence theorem that

$$\lim_{k\to\infty} \|\tbinom{1}{v} \cdot \nabla_z (f_\varepsilon - f_{\varepsilon,k})\|_{L^2(\Omega_{t,x};V')} \le \lim_{k\to\infty} \|\tbinom{1}{v} \cdot \nabla_z (f_\varepsilon - f_{\varepsilon,k})\|_{L^2(\Omega_{t,x};L^2(\Omega_v))} = 0.$$

Hence, $f_{\varepsilon,k}$ converges to $f_\varepsilon$ in $H^1_{\mathrm{FP}}(\Omega)$, which completes the proof of proposition 3.1. □

## S2. Discussion about trace theorems

As already mentioned in section 3, we believe that the statement in assumption 4.4 is still an open problem, despite the fact that more general results implying the respective version of assumption 4.4 hold true for $L^2$-based spaces, and that similar results for Fokker-Planck equations are given in other works.

More precisely, on the one hand, [S1, Lemma 4.5] states that the space $C_0^\infty(\bar{\Omega}\backslash\Gamma_0)$ of smooth functions vanishing in a neighborhood of $\Gamma_0$ is dense in $H^1_{\mathrm{FP}}(\Omega)$, and that $H^1_{\mathrm{FP}}(\Omega)$ functions lying in $L^2(\Gamma_+, |(1,v)^T \cdot n|)$ or $L^2(\Gamma_-, |(1,v)^T \cdot n|)$ already have a full global trace in $L^2(\partial\Omega, |(1,v)^T \cdot n|)$.

On the other hand, in [S4], and based on that also in [S2] the following is stated[1]:

**Claim S2.1** (cf. [S4, Lemma 2.3], [S2, p. 3493])**.** *Let $w \in H^1_{\mathrm{FP}}(\Omega)$. Then, $w \in L^2(\Gamma_\pm, |(1,v)^T \cdot n|)$ and the integration by parts formula* (26) *holds.*

[1]In describing the estimates in different cited works, we substitute the notation and the concrete spaces to the respective equivalent in this work to simplify the discussion. This sometimes slightly changes the spaces, but has no effect on the used arguments.

Note, that [S1, Lemma 4.5] would already imply assumption 4.4 (where functions that have zero trace on $\Gamma_-$ are considered), while claim S2.1 is an even stronger claim. However, we believe that the arguments both for [S1, Lemma 4.5] and for claim S2.1 given in [S1, S4, S2] are incomplete.

While the function spaces considered for the different versions of the Fokker-Planck equation are typically of the form

$$H^1_{\mathrm{FP}}(\Omega) = \{w \in \mathcal{X} : \left(\begin{smallmatrix}1\\v\end{smallmatrix}\right) \cdot \nabla_{t,x} w \in \mathcal{X}'\} \text{ with } \mathcal{X} = L^2(\Omega_{t,x}, H^1(\Omega_v)),$$

function spaces for other kinetic equations like neutron transport require considering

$$H^1_{\mathrm{NT}}(\Omega) = \{w \in L^2(\Omega) : \left(\begin{smallmatrix}1\\v\end{smallmatrix}\right) \cdot \nabla_{t,x} w \in L^2(\Omega)\}.$$

Properties of $H^1_{\mathrm{NT}}(\Omega)$ have been studied in many previous works ([S3, S5], for a summary see [S7, Chap. XXI]) and many techniques can be used similarly for $H^1_{\mathrm{FP}}(\Omega)$, e.g., proposition 3.2. We note that while the statement of [S1, Lemma 4.5] and thus of assumption 4.4 holds for $H^1_{\mathrm{NT}}(\Omega)$ instead of $H^1_{\mathrm{FP}}(\Omega)$ (see [S3, S5, S6],[S7, Chap. XXI]), claim S2.1 is not true for $H^1_{\mathrm{NT}}(\Omega)$ functions, see e.g. [S7, Chap. XXI, Remark 3] and [S10, pp. 562-563] for an example for a function in $H^1_{\mathrm{NT}}(\Omega)$ that does not have traces in $L^2(\Gamma_\pm\,|(1,v)^T \cdot n|)$.

The argument to show claim S2.1 in [S4] is based on two steps:

*Step 1:* Show that the space $C_0^\infty(\bar{\Omega} \setminus \Gamma_0)$ is dense in $H^1_{\mathrm{FP}}(\Omega)$ (as also included in [S1, Lemma 4.5])

*Step 2:* Decompose $w \in C_0^\infty(\bar{\Omega} \setminus \Gamma_0)$ into $w = w_+ + w_-$ with $w_\pm$ vanishing on $\Gamma_\pm$ and use the density from *Step 1* to show the claim.

We believe the arguments in both steps to be incomplete.

For *Step 1*, the author of [S4] refers to [S8], where a time-dependent Fokker-Planck equation in one space dimension is considered and where it is stated that using an argument of Bardos ([S3, p. 203]), it can be seen that $C_0^\infty(\bar{\Omega} \setminus \Gamma_0)$ is dense in $H^1_{\mathrm{FP}}(\Omega)$.

The work of Bardos [S3] considers $L^2$-based function spaces as e.g. $H^1_{\mathrm{NT}}(\Omega)$. In [S3, pp. 202-203], a family of functions $(\varphi_\delta)_{\delta>0} \subset C^\infty(\bar{\Omega})$ is constructed such that $\varphi_\delta$ vanishes in the $\delta$-neighborhood of $\partial\Gamma_-$, and is equal to unity outside of the $2\delta$-neighborhood. Given $u \in H^1_{\mathrm{NT}}(\Omega) \cap L^\infty(\Omega)$, it is then shown that $u\varphi_\delta \to u$ in $L^2(\Omega)$ and $\left(\begin{smallmatrix}1\\v\end{smallmatrix}\right) \cdot \nabla_{t,x}(u\varphi_\delta) \to \left(\begin{smallmatrix}1\\v\end{smallmatrix}\right) \cdot \nabla_{t,x} u$ in $L^2(\Omega)$ as $\delta \to 0$. The estimate of $\|u\left(\begin{smallmatrix}1\\v\end{smallmatrix}\right) \cdot \nabla_{t,x}\varphi_\delta\|_{L^2(\Omega)}$, uses the fact that $|\nabla\varphi_\delta| < C\delta^{-1}$ while $\operatorname{supp}\varphi_\delta$ has a measure bounded by $C\delta$ and $u \in L^\infty(\Omega)$.

Subsequently, in [S3] this density result is used to show that functions with vanishing trace on $\Gamma_-$ can be approximated by smooth functions that vanish on $\Gamma_-$.

To use the same approach for $H^1_{\mathrm{FP}}(\Omega)$, one needs to show that $\|u - u\varphi_\delta\|_{H^1_{\mathrm{FP}}(\Omega)} \to 0$ as $\delta \to 0$, which has not been addressed in [S8, S4]. The convergence of $\|u - u\varphi_\delta\|_{\mathcal{X}}$ can indeed be shown analogously to the proof in [S3], since the additional term $\|\nabla_v(u - u\varphi_\delta)\|_{L^2(\Omega)}$ can be treated exactly as the $L^2$-derivative term in [S3], see also [S1].

However, it is unclear to us how to show convergence (or even boundedness independently of $\delta$) for $\|\left(\begin{smallmatrix}1\\v\end{smallmatrix}\right) \cdot \nabla_{t,x}(u - u\varphi_\delta)\|_{\mathcal{X}'}$. Instead of $L^2$-norms, here it is required to have an estimate of the form

$$\langle \varphi_\delta \left(\begin{smallmatrix}1\\v\end{smallmatrix}\right) \cdot \nabla_{t,x} u, \psi \rangle_{\mathcal{X}',\mathcal{X}} = \langle \left(\begin{smallmatrix}1\\v\end{smallmatrix}\right) \cdot \nabla_{t,x} u, \varphi_\delta \psi \rangle_{\mathcal{X}',\mathcal{X}} \le C(u)\|\psi\|_{\mathcal{X}} \quad \forall \psi \in \mathcal{X}.$$

Unfortunately, we do not know how to obtain such an estimate. Note, that $\|\varphi_\delta \psi\|_{\mathcal{X}}$ cannot be bounded analogously to the proof of [S3], since generally $\psi \notin L^\infty(\Omega)$. We therefore do not see how to obtain a bound of $\|\varphi_\delta \psi\|_{\mathcal{X}}$ independently of $\delta$ as claimed in [S1]. Therefore, it is unclear to us if and how the approach for $H^1_{\mathrm{NT}}(\Omega)$ can be transferred to $H^1_{\mathrm{FP}}(\Omega)$ to show assumption 4.4, [S1, Lemma 4.5], and *Step 1* in the proof of claim S2.1 by [S4].

In *Step 2* to prove claim S2.1, the authors of [S4, S2] decompose a function $\psi \in C_0^\infty(\bar{\Omega} \setminus \Gamma_0)$ into a sum $\psi = \psi_+ + \psi_-$, where $\psi_\pm \in C^\infty(\bar{\Omega})$ vanish on $\Gamma_\pm$. Using integration by parts separately for $\psi_\pm$, one can show that

$$\|\psi_+\|_{L^2(\Gamma_-,|(1,v)^T\cdot n|)} \leq C\|\psi_+\|_{H^1_{\mathrm{FP}}(\Omega)} \quad \text{and} \quad \|\psi_-\|_{L^2(\Gamma_+,|(1,v)^T\cdot n|)} \leq C\|\psi_-\|_{H^1_{\mathrm{FP}}(\Omega)}.$$

The authors conclude from this that $\|\psi\|_{L^2(\Gamma_+\cup\Gamma_-,|(1,v)^T\cdot n|)} \leq C\|\psi\|_{H^1_{\mathrm{FP}}(\Omega)}$. However, as already noted in [S1, Appendix], it is not clear if this conclusion holds for a constant $C$ independently of $\psi$, since the decomposition actually leads to

$$\|\psi\|_{L^2(\Gamma_+\cup\Gamma_-,|(1,v)^T\cdot n|)} \leq C(\|\psi_+\|_{H^1_{\mathrm{FP}}(\Omega)} + \|\psi_-\|_{H^1_{\mathrm{FP}}(\Omega)}). \tag{S2}$$

It is unclear to us whether $\psi_+$ and $\psi_-$ can be chosen in such a way that their single norms can be bounded from above by $\|\psi\|_{H^1_{\mathrm{FP}}(\Omega)}$, see also the discussion in [S1].

We emphasize again that claim S2.1 does not hold for $H^1_{\mathrm{NT}}(\Omega)$, as demonstrated by the counterexample in [S10, pp. 562-563]. Since $H^1_{\mathrm{FP}}(\Omega)$ functions have additional regularity in the velocity variable, one cannot conclude from the $H^1_{\mathrm{NT}}(\Omega)$ case that claim S2.1 must be false. However, we conjecture that a proof of claim S2.1 has to rely on this additional regularity to exploit the difference between the spaces.

To summarize, we believe the arguments in [S1, S4, S2] to be incomplete. Moreover, we do not know how to use ideas from the existing approaches for $H^1_{\mathrm{NT}}(\Omega)$ to show assumption 4.4, since we are unsure how to compensate for the missing $L^2$ regularity of the transport term even with a higher regularity in the velocity direction. Therefore, we leave assumption 4.4 as an open problem.

## References


[S1] S. Armstrong and J.-C. Mourrat, *Variational methods for the kinetic Fokker-Planck equation*, Feb. 2019, https://arxiv.org/abs/1902.04037v1.

[S2] G. Bal and B. Palacios, *Pencil-beam approximation of stationary Fokker-Planck*, SIAM J. Math. Anal., 52 (2020), pp. 3487–3519, https://doi.org/10.1137/19M1295775.

[S3] C. Bardos, *Problèmes aux limites pour les équations aux dérivées partielles du premier ordre à coefficients réels; théorèmes d'approximation; application à l'équation de transport*, Ann. Sci. École Norm. Sup. (4), 3 (1970), pp. 185–233, https://doi.org/10.24033/asens.1190.

[S4] J. A. Carrillo, *Global weak solutions for the initial-boundary-value problems to the Vlasov-Poisson-Fokker-Planck system*, Math. Methods Appl. Sci., 21 (1998), pp. 907–938, https://doi.org/10.1002/(SICI)1099-1476(19980710)21:10<907::AID-MMA977>3.3.CO;2-N.

[S5] M. Cessenat, *Théorèmes de trace $L^p$ pour des espaces de fonctions de la neutronique*, C. R. Acad. Sci. Paris Sér. I Math., 299 (1984), pp. 831–834.

[S6] M. Cessenat, *Théorèmes de trace pour des espaces de fonctions de la neutronique*, C. R. Acad. Sci. Paris Sér. I Math., 300 (1985), pp. 89–92.

[S7] R. Dautray and J.-L. Lions, *Mathematical analysis and numerical methods for science and technology. Vol. 6*, Springer-Verlag, Berlin, 1993, https://doi.org/10.1007/978-3-642-58004-8. Evolution problems. II.

[S8] P. Degond and S. Mas-Gallic, *Existence of solutions and diffusion approximation for a model Fokker-Planck equation*, in Proceedings of the conference on mathematical methods applied to kinetic equations (Paris, 1985), vol. 16, 1987, pp. 589–636, https://doi.org/10.1080/00411458708204307.

[S9] E. Hebey, *Nonlinear Analysis on Manifolds: Sobolev Spaces and Inequalities*, Courant lecture notes in mathematics, Courant Institute of Mathematical Sciences, 2000.

[S10] T. A. Manteuffel, K. J. Ressel, and G. Starke, *A boundary functional for the least-squares finite-element solution of neutron transport problems*, SIAM J. Numer. Anal., 37 (2000), pp. 556–586, https://doi.org/10.1137/S0036142998344706.

University of Münster, Applied Mathematics, Einsteinstr. 62, 48149 Münster, Germany, julia.brunken@uni-muenster.de

University of Twente, Faculty of Electrical Engineering, Mathematics & Computer Science, Zilverling, P.O. Box 217, 7500 AE Enschede, The Netherlands. Current address: Department of Mathematical Sciences, Stevens Institute of Technology, 1 Castle Point Terrace, Hoboken, NJ 07030, United States of America, ksmetana@stevens.edu.
